# Supplementary material for: Better Parameter-free Stochastic Optimization with ODE Updates for Coin-Betting
Source: arXiv:2006.07507 source file (2022-05-03)
Supplement: Supplementary file 1 [file appendix.tex]

\section{Appendix}
\label{sec:appendix}

\subsection{Proof of Improved Guarantee of equation~\ref{eq:coin2}}
We start from the coin-betting proof. The reduction from coin-betting to optimization goes as described in Section~\ref{sec:def}, that is through a guaranteed wealth lower bound. Hence, consider the generalized betting game with vectorial coins. For the rounds in which $\bg_t$ is zero, there is no change on the wealth, regardless of the money the gambler bets. Hence, we can safely discard these rounds from the betting game and nothing would change in terms of wealth. On the other hand, the betting fraction given by KT would change because $t$ would be substituted by the number of non-zero rounds up to that moment. Also, the total length of the game would change from $T$ to $\sum_{t=1}^T \boldsymbol{1}[\bg_t\neq\boldsymbol{0}]$.
Hence, we can directly take the update in \eqref{eq:coin} and substitute $t$ with $\sum_{j=1}^t \boldsymbol{1}[\bg_j\neq\boldsymbol{0}]$ and the regret upper bound that is $O\left(\sqrt{T}\right)$ to $O\left(\sqrt{\sum_{t=1}^T \boldsymbol{1}[\bg_t\neq\boldsymbol{0}]}\right)$. Finally, standard online-to-batch conversion~\citep{Cesa-BianchiCG04} gives the stated rate.

\subsection{List of Datasets}
We performed experiments with 21 different machine learning binary classification datasets and 17 regression datasets from the LIBSVM website~\citep{ChangL01} and OpenML\citep{OpenML2013}, see Table~\ref{table:datasets} for details on the datasets. For OpenML datasets, categorical features are converted to numerical ones with a one-hot encoding.

\begin{table}[!h]
\caption{Datasets for experiments. ($1^{st}$) Regression datasets, ($2^{nd}$) Classification datasets.}
\label{table:datasets} 
\begin{minipage}{\linewidth}
  \centering
	\begin{tabular}{p{0.35\textwidth}p{0.2\textwidth}rp{0.15\textwidth}}
	\toprule
	Dataset Name & Training size & \# of features \\
	\midrule
	abalon   &4,177  & 8  \\
	cadata &20640 &8\\
	cpusmall &8192 &12\\
	gisette &6,000 &5,000\\
	mg &1385 &6\\
	space-ga &3,107 &6\\
	visualizing-soil &8,641 &4\\
	cpu-act &8,192 &21\\
	delta-elevator &9,517 &6\\
	wind &6,574 &14\\
	bank32nh &8,192 &32\\
	houses &20,640 &8\\
	houses-8L &22,784 &8\\
	diamonds &53,974 &9\\
	fried &40,768 &10\\
	rainfall &16,755 &3\\
	BNG(stock) &59,049 &9\\
	BNG(pwLinear) &177,147 &10\\
	\bottomrule
	\end{tabular}
\end{minipage}
\quad \quad
\begin{minipage}{\linewidth}
  \centering
	\begin{tabular}{p{0.35\textwidth}p{0.2\textwidth}rp{0.15\textwidth}}
	\toprule
	Dataset Name & Training size & \# of features \\
	\midrule
	a9a       &32,561& 123\\
	mushrooms &8,124 &112\\
	w8a &49,749 &300\\
	phishing &11,055 &68\\
	ijcnn1 &49,990 &22\\
	coil2000 &9,822 &85\\
	mammography &11,183 &6\\
	abalone &4,177 &8\\
	2dplane &40,768 &10\\
	ailerons &13,750 &41\\
	cpu-act &8,192 &21\\
	data-ailerons & 7,129 &5\\
	kin8nm &8,192 &8\\
	delta-elevator &9,517 &6\\
	house-16H &22,784 &16\\
	cal-housing &20,640 &8\\
	houses &20,640 &8\\
	bank32nh &8,192 &32\\
	house-8L &22,784 &8\\
	fried &40,768 &10\\
	\bottomrule
	\end{tabular}
\end{minipage}	
\end{table}

\subsection{Additional Details of Real Datasets Experiments}
In Section~\ref{sec:exp}, we test the ability of CODE to get a good generalization error in real datasets tasks. We normalize each instance to have norm $\sqrt{2}/2$ and augment the features with a constant bias term of $\sqrt{2}/2$, so that the norm of the augmented samples is 1. To choose the initial step size for the regression and classification tasks with the grid $10^{\{-2.5:0.5:5\}}$ for SGD, SGD with truncated models, SGD with Importance Weight Aware updates, AdaGrad, and Adam. CODE, Coin, and Recursive have no parameters to tune.

\subsection{Additional Data Analysis}
We report best fixed learning rates in Table~\ref{table:best_lr}. For each algorithm, the number in Table~\ref{table:best_lr} is the optimal learning rate that achieves the best average of normalized performance over all datasets directly on the test sets. Note that best fixed learning rates are not at the border of the grid of learning rates.

\begin{table}[h]
\caption{Best fixed learning rates. (Left) Regression tasks, (Right) Classification tasks.}
\label{table:best_lr} 
\begin{minipage}{.45\linewidth}
  \centering
	\begin{tabular}{p{0.35\textwidth}p{0.35\textwidth}}
	\toprule
	Algorithm & Best fixed lr\\
	\midrule
	SGD   &$1$  \\
	IWA &$10^{}$ \\
	aProx &$10^{3}$ \\
	AdaGrad &$1$ \\
	Adam &$10^{-1.5}$ \\
	\bottomrule
	\end{tabular}
\end{minipage}
\quad \quad
\begin{minipage}{.45\linewidth}
  \centering
	\begin{tabular}{p{0.35\textwidth}p{0.35\textwidth}}
	\toprule
	Algorithm & Best fixed lr\\
	\midrule
	SGD &$10$  \\
	IWA &$10$ \\
	aProx &$10$ \\
	AdaGrad &$10^{0.5}$ \\
	Adam &$10^{-1.5}$\\
	\bottomrule
	\end{tabular}
\end{minipage}
\end{table}

We also studied how does the performance of each algorithm depend on learning rate tuning with real datasets. For each dataset, we take the average of test loss over 3 repetitions and plot the averaged test losses versus the corresponding learning rates. There is no learning rate to tune for CODE, Coin, and Recursive, so we just plot a horizontal line of test loss for both of them. In Figures~\ref{fig:te_versus_lr} and~\ref{fig:te_versus_lr1}, we can see that the baseline algorithms are sensitive to step sizes. Only with a limited number of step size choices, the baseline algorithms are competitive to CODE. As we discussed above, the tuning procedure is computationally expensive. Still, CODE achieved almost optimal performance without anything to tune. 

\subsection{Additional synthetic experiments}
In Section~\ref{sec:exp}, we generated synthetic datasets and considered regression problem. We also consider the classification setting, generating the inputs as in Section~\ref{sec:exp}, setting the labels to $\by=\sign(A \bx^\star)$, and discarding samples to guarantee a margin of 0.05. In the noisy-case, we flipped a fraction of the labels at random. We used the average empirical hinge loss as the function $F(\bx)$. Figure~\ref{fig:hinge_clean} shows again the number of iterations to reach sub-optimality of 0.05. We can see that in the classification setting the behaviours of the algorithms mirrors the regression case. So, IWA and aProx have an advantage in the noise-free case over SGD that shrinks in the noisy case, and again \emph{CODE gives essentially optimal performance without any tuning}.

\begin{figure}[!h]
\centering 
\includegraphics[width=.49\textwidth]{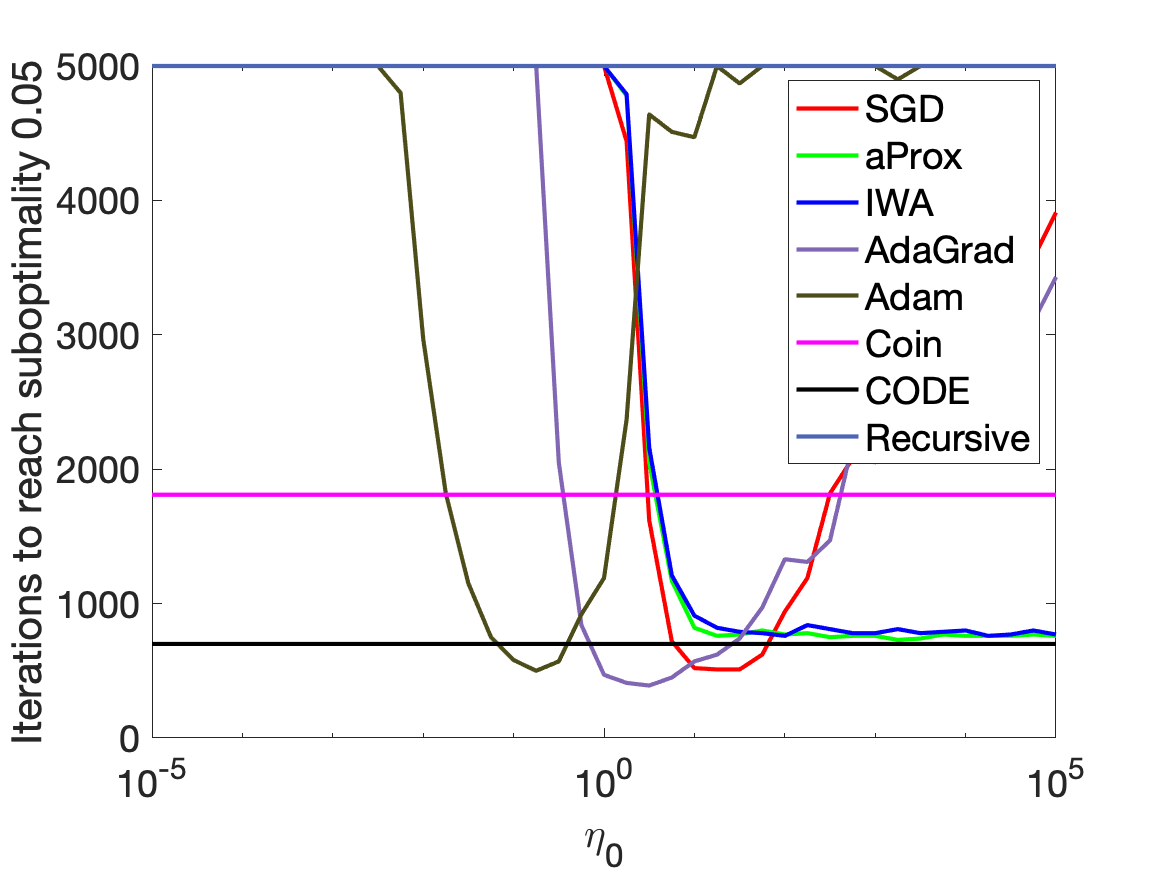}
\includegraphics[width=.49\textwidth]{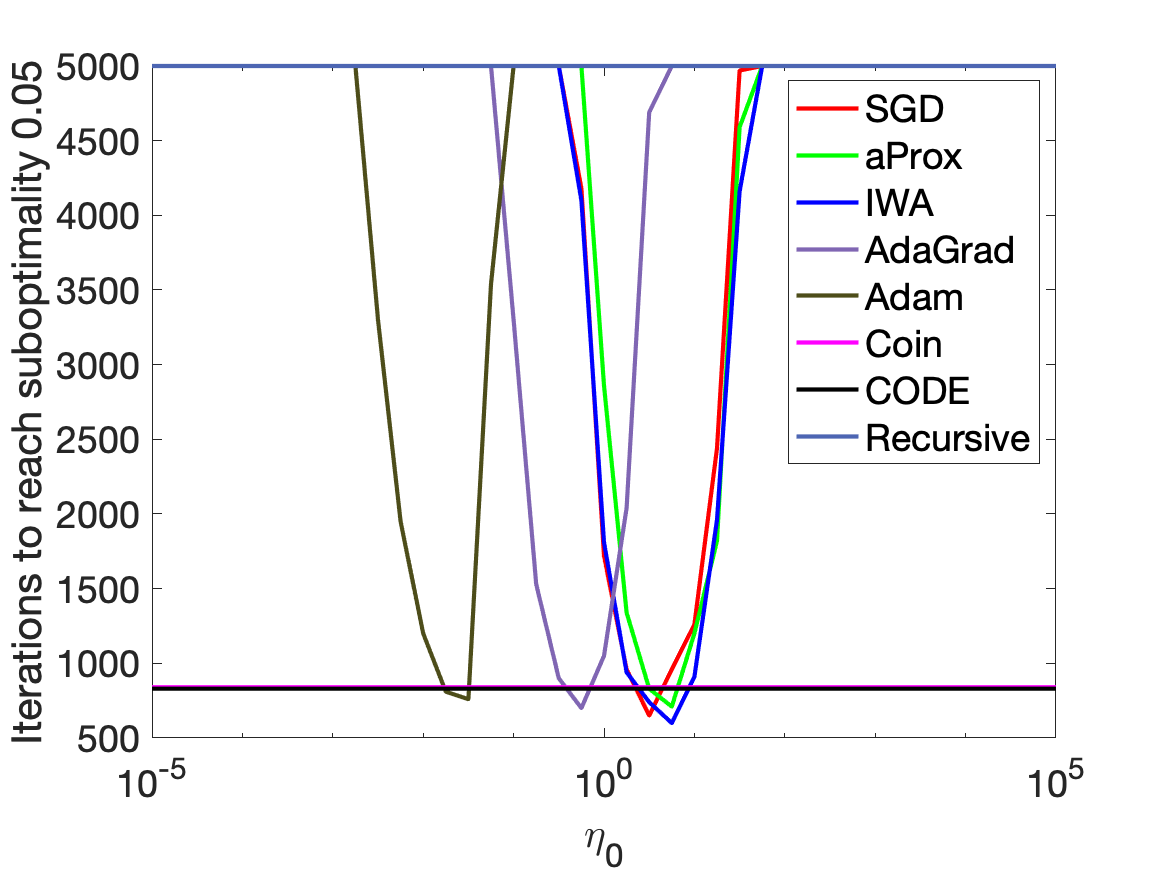}
\caption{Synthetic dataset with hinge loss. Number of iteration to reach $0.05$ suboptimality gap versus initial step sizes $\eta_0$. ($1^{st}$) noiseless setting, ($2^{nd}$) 20\% of the labels flipped at random.}
\label{fig:hinge_clean}
\end{figure}

\onecolumn
\centering
\begin{figure}[b]
\centering
\includegraphics[width=4.9cm]{70tr_15val_15te/te_loss_vs_lr/a9a_te_loss_vs_lr} \hfill
\hspace{-0.6cm}
\includegraphics[width=4.9cm]{70tr_15val_15te/te_loss_vs_lr/ijcnn1_no_yaxis_te_loss_vs_lr} 
\hfill
\hspace{-0.6cm}
\includegraphics[width=4.9cm]{70tr_15val_15te/te_loss_vs_lr/mushrooms_no_yaxis_te_loss_vs_lr} \hfill
\vspace{-0.5cm}
\includegraphics[width=4.9cm]{70tr_15val_15te/te_loss_vs_lr/phishing_te_loss_vs_lr} \hfill\hspace{-0.6cm}
\includegraphics[width=4.9cm]{70tr_15val_15te/te_loss_vs_lr/w8a_no_yaxis_te_loss_vs_lr} \hfill\hspace{-0.6cm}
\includegraphics[width=4.9cm]{70tr_15val_15te/te_loss_vs_lr/ds_298_2_no_yaxis_te_loss_vs_lr} \hfill
\vspace{-0.5cm}
\includegraphics[width=4.9cm]{70tr_15val_15te/te_loss_vs_lr/ds_310_2_te_loss_vs_lr} \hfill\hspace{-0.6cm}
\includegraphics[width=4.9cm]{70tr_15val_15te/te_loss_vs_lr/ds_720_2_no_yaxis_te_loss_vs_lr} \hfill\hspace{-0.6cm}
\includegraphics[width=4.9cm]{70tr_15val_15te/te_loss_vs_lr/ds_727_2_no_yaxis_te_loss_vs_lr} \hfill
\vspace{-0.5cm}
\includegraphics[width=4.9cm]{70tr_15val_15te/te_loss_vs_lr/ds_734_2_te_loss_vs_lr} \hfill\hspace{-0.6cm}
\includegraphics[width=4.9cm]{70tr_15val_15te/te_loss_vs_lr/ds_761_2_no_yaxis_te_loss_vs_lr} \hfill\hspace{-0.6cm}
\includegraphics[width=4.9cm]{70tr_15val_15te/te_loss_vs_lr/ds_803_2_no_yaxis_te_loss_vs_lr} \hfill
\vspace{-0.5cm}
\includegraphics[width=4.9cm]{70tr_15val_15te/te_loss_vs_lr/ds_807_2_te_loss_vs_lr} \hfill\hspace{-0.6cm}
\includegraphics[width=4.9cm]{70tr_15val_15te/te_loss_vs_lr/ds_816_2_no_yaxis_te_loss_vs_lr} \hfill\hspace{-0.6cm}
\includegraphics[width=4.9cm]{70tr_15val_15te/te_loss_vs_lr/ds_819_2_no_yaxis_te_loss_vs_lr} \hfill
\vspace{-0.5cm}
\includegraphics[width=4.9cm]{70tr_15val_15te/te_loss_vs_lr/ds_821_2_te_loss_vs_lr} \hfill\hspace{-0.6cm}
\includegraphics[width=4.9cm]{70tr_15val_15te/te_loss_vs_lr/ds_822_2_no_yaxis_te_loss_vs_lr} \hfill\hspace{-0.6cm}
\includegraphics[width=4.9cm]{70tr_15val_15te/te_loss_vs_lr/ds_823_2_no_yaxis_te_loss_vs_lr} \hfill
\vspace{-0.5cm}
\includegraphics[width=4.9cm]{70tr_15val_15te/te_loss_vs_lr/ds_833_2_te_loss_vs_lr} \hfill\hspace{-0.6cm}
\includegraphics[width=4.9cm]{70tr_15val_15te/te_loss_vs_lr/ds_843_2_no_yaxis_te_loss_vs_lr} \hfill\hspace{-0.6cm}
\includegraphics[width=4.9cm]{70tr_15val_15te/te_loss_vs_lr/ds_901_2_no_yaxis_te_loss_vs_lr} \hfill\hfill
\caption{Test loss vs learning rate (Classification Results).}
\label{fig:te_versus_lr}
\end{figure}

\begin{figure}[b]
\centering
\includegraphics[width=4.9cm]{70tr_15val_15te/te_loss_vs_lr/abalone_te_loss_vs_lr} \hfill\hspace{-0.6cm}
\includegraphics[width=4.9cm]{70tr_15val_15te/te_loss_vs_lr/cadata_no_yaxis_te_loss_vs_lr} \hfill\hspace{-0.6cm}
\includegraphics[width=4.9cm]{70tr_15val_15te/te_loss_vs_lr/cpusmall_no_yaxis_te_loss_vs_lr} \hfill
\vspace{-0.5cm}
\includegraphics[width=4.9cm]{70tr_15val_15te/te_loss_vs_lr/space_ga_te_loss_vs_lr} \hfill\hspace{-0.6cm}
\includegraphics[width=4.9cm]{70tr_15val_15te/te_loss_vs_lr/mg_no_yaxis_te_loss_vs_lr} \hfill\hspace{-0.6cm}
\includegraphics[width=4.9cm]{70tr_15val_15te/te_loss_vs_lr/ds_688_41_no_yaxis_te_loss_vs_lr} \hfill
\vspace{-0.5cm}
\includegraphics[width=4.9cm]{70tr_15val_15te/te_loss_vs_lr/ds_573_100_te_loss_vs_lr} \hfill\hspace{-0.6cm}
\includegraphics[width=4.9cm]{70tr_15val_15te/te_loss_vs_lr/ds_198_1_no_yaxis_te_loss_vs_lr} \hfill\hspace{-0.6cm}
\includegraphics[width=4.9cm]{70tr_15val_15te/te_loss_vs_lr/ds_503_43_no_yaxis_te_loss_vs_lr} \hfill
\vspace{-0.5cm}
\includegraphics[width=4.9cm]{70tr_15val_15te/te_loss_vs_lr/ds_558_1_te_loss_vs_lr} \hfill\hspace{-0.6cm}
\includegraphics[width=4.9cm]{70tr_15val_15te/te_loss_vs_lr/ds_537_500002_2_no_yaxis_te_loss_vs_lr} \hfill\hspace{-0.6cm}
\includegraphics[width=4.9cm]{70tr_15val_15te/te_loss_vs_lr/ds_218_500002_no_yaxis_te_loss_vs_lr} \hfill
\vspace{-0.5cm}
\includegraphics[width=4.9cm]{70tr_15val_15te/te_loss_vs_lr/ds_42225_18824_te_loss_vs_lr} \hfill\hspace{-0.6cm}
\includegraphics[width=4.9cm]{70tr_15val_15te/te_loss_vs_lr/ds_564_31_no_yaxis_te_loss_vs_lr} \hfill\hspace{-0.6cm}
\includegraphics[width=4.9cm]{70tr_15val_15te/te_loss_vs_lr/ds_41539_3002_no_yaxis_te_loss_vs_lr} \hfill
\vspace{-0.5cm}
\includegraphics[width=4.9cm]{70tr_15val_15te/te_loss_vs_lr/ds_1200_64_te_loss_vs_lr} \hfill \hspace{-0.6cm}
\includegraphics[width=4.9cm]{70tr_15val_15te/te_loss_vs_lr/ds_1203_16_no_yaxis_te_loss_vs_lr} \hfill\hfill \hfill \hfill \hfill \hfill \hfill
\caption{Test loss vs learning rate (Regression Results).}
\label{fig:te_versus_lr1}
\end{figure}
